# Supplementary material for: JaxNet: Scalable Blockchain Network
Source: arXiv:2005.01865 source file (2020-10-28)
Supplement: Supplementary file 1 [file RecentPaperOnEfficiency.tex]

\subsection{Recent paper}

In the recent paper by Yo-Der Song and Tomaso Aste \cite{song2020cost}
